# Supplementary material for: Relation Extraction in underexplored biomedical domains: A diversity-optimised sampling and synthetic data generation approach
Source: arXiv:2311.06364 source file (2023-11-10)
Supplement: Supplementary file 2 [file supptables.tex]

\section{Supplementary tables}
